# Supplementary material for: High pressure and temperature thermoelasticity of hcp osmium from ab initio quasi-harmonic theory
Source: arXiv:2507.15354 source file (2025-07-21)
Supplement: Supplementary file 1 [file Supplementary_file.pdf]

# Supplementary material for: High pressure and temperature thermoelasticity of hcp osmium from ab initio quasi-harmonic theory

Xuejun Gong\*

*School of Physical Science and Technology, Xinjiang University, Urumqi, Xinjiang 830046, China and  
International School for Advanced Studies (SISSA), Via Bonomea 265, 34136, Trieste, Italy*

Andrea Dal Corso†

*International School for Advanced Studies (SISSA), Via Bonomea 265, 34136, Trieste, Italy and  
IOM - CNR, Via Bonomea 265, 34136, Trieste, Italy*

(Dated: June 23, 2025)

We present the thermal expansion, isobaric heat capacity, and adiabatic bulk modulus of osmium at elevated temperatures and pressures, calculated using the Perdew-Burke-Ernzerhof (PBE) exchange-correlation functional. Comparative data from experiments are included for reference. Figures illustrating temperature-dependent elastic constants (TDECs) are provided, wherein our predictions are directly compared with experimental results without any applied offset to the 0 K values. We also contrast quasi-harmonic approximation (QHA) elastic constants calculated with and without the contribution of electronic excitations in the free energy. Finally, we demonstrate the convergence of elastic constants with respect to  $\mathbf{k}$ -point sampling.

Table I presents the lattice parameter  $a$  and the  $c/a$  ratio along the stress-pressure curve. The corresponding pressure and volume values for each data point are also included. The temperature-dependent elastic constants (TDECs) were computed utilizing geometries 2, 4, 5, 6, and 7 as equilibrium configurations, resulting in a maximum considered pressure of 1604 kbar.

Fig. 1 illustrates the two independent components of the thermal expansion tensor,  $\alpha_{xx}$  and  $\alpha_{zz}$ , along with the volumetric thermal expansion,  $\beta$ , calculated at 0 kbar. These quantities were derived from the temperature-dependent lattice parameters,  $a(T)$  and  $c/a(T)$ , obtained through free energy minimization on a two-dimensional grid. The volumetric thermal expansion calculated directly from the volume,  $V(T)$ , minimized on the stress-pressure curve geometries, is also presented (green line). As observed, this result is nearly indistinguishable from that derived from the thermal expansion tensor. At variance with previous calculations reported

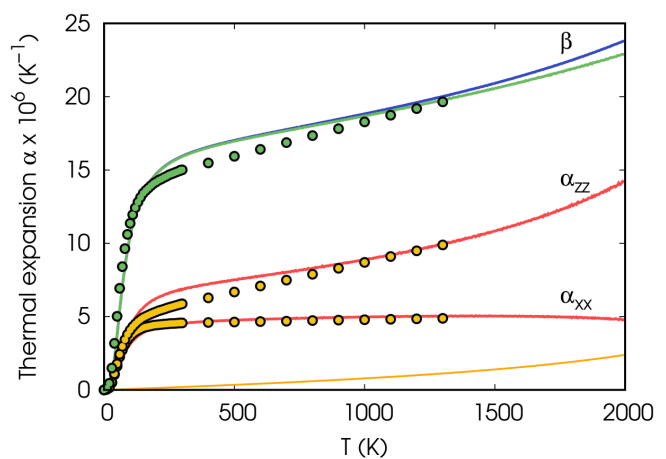

FIG. 1. PBE temperature variation of the thermal expansion. The two red lines shows the linear thermal expansion tensor components  $\alpha_{xx}$  and  $\alpha_{zz}$  obtained using the two dimensional grid of  $a$  and  $c/a$  values. The volume thermal expansion  $\beta$  (blue line) is obtained as  $\beta = 2\alpha_{xx} + \alpha_{zz}$ . The green line is the volume thermal expansion obtained from the free energy calculated along the stress-pressure curve. The experimental data (green and yellow dots) are those summarized in Ref. [1]. The orange line shows the electronic contribution to the volume thermal expansion.

TABLE I. The 0 K “stress-pressure” curve. In the configurations with \* we have computed the QHA TDECs. For all other values of pressure and temperature we have interpolated them.

| geometry | pressure (kbar) | $a$ (a.u.) | $c/a$ | Volume (a.u.) <sup>3</sup> |
|----------|-----------------|------------|-------|----------------------------|
| 1        | 2320            | 4.70       | 1.597 | 143.51                     |
| 2*       | 1604            | 4.80       | 1.593 | 152.53                     |
| 3        | 1039            | 4.90       | 1.589 | 161.92                     |
| 4*       | 601             | 5.00       | 1.586 | 171.67                     |
| 5*       | 265             | 5.10       | 1.582 | 181.74                     |
| 6*       | 9               | 5.20       | 1.578 | 192.15                     |
| 7*       | −182            | 5.30       | 1.573 | 202.87                     |

\* xuejun.gong@xju.edu.cn

† dalcorso@sissa.it

in Ref. [2], the present study incorporates the contribution of electronic excitations to the free energy. The electronic contribution to the volumetric thermal expansion is depicted in orange in Fig. 1. This contribution is negligible up to approximately 1000 K, but becomes significant at higher temperatures. Notably, inclusion of electronic excitations improves the agreement with experimental data.

Fig. 2 displays the volumetric thermal expansion as a function of temperature for four distinct pressures: 0

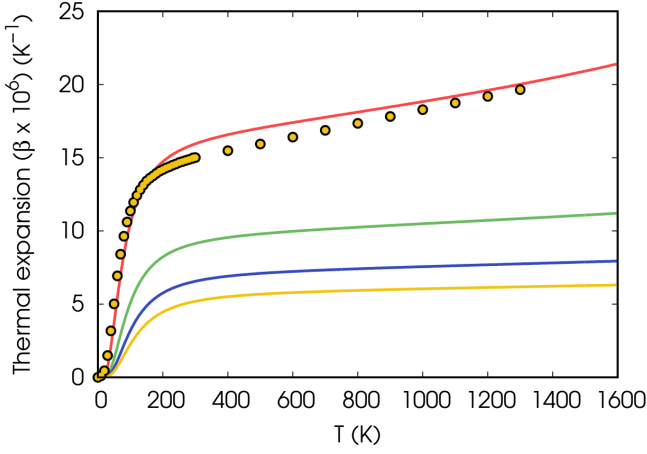

FIG. 2. PBE temperature variation of the volume thermal expansion at several pressures: 0 kbar red, 500 kbar green, 1000 kbar blue, 1500 kbar yellow. The experimental data (yellow dots) are from Ref. [1].

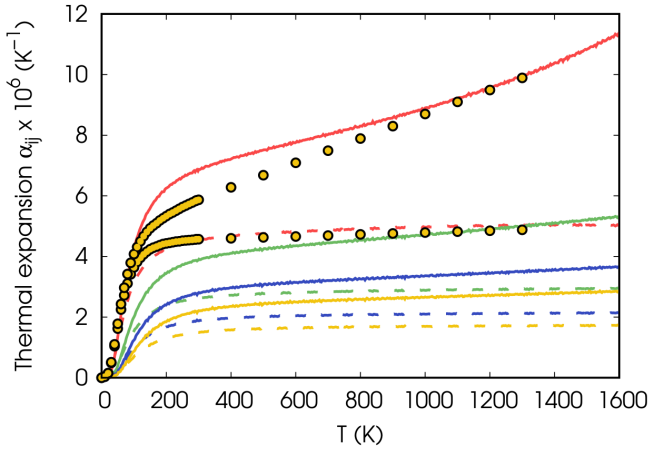

FIG. 3. PBE temperature variation of the thermal expansion tensor at several pressures: 0 kbar red, 500 kbar green, 1000 kbar blue, 1500 kbar yellow. The continuous lines show the  $\alpha_{zz}$  component, while the dashed lines show the  $\alpha_{xx}$  component. The experimental data (yellow dots) are from Ref. [1].

kbar, 500 kbar, 1000 kbar, and 1500 kbar. Fig. 3 shows the temperature dependence of the thermal expansion tensor components at the same pressures. As observed, the difference between  $\alpha_{xx}$  and  $\alpha_{zz}$  diminishes with increasing pressure, indicating a trend toward isotropic behavior.

Fig. 4 presents the isobaric heat capacity as a function of temperature at various pressures, alongside experimental data from Ref. [1] at zero pressure. Consistent with findings reported in Ref. [2], with the inclusion of electronic excitations in the heat capacity calculations QHA accurately reproduces experimental results up to 1300 K, suggesting a minimal role for anharmonic phonon-phonon interactions in osmium within this temperature

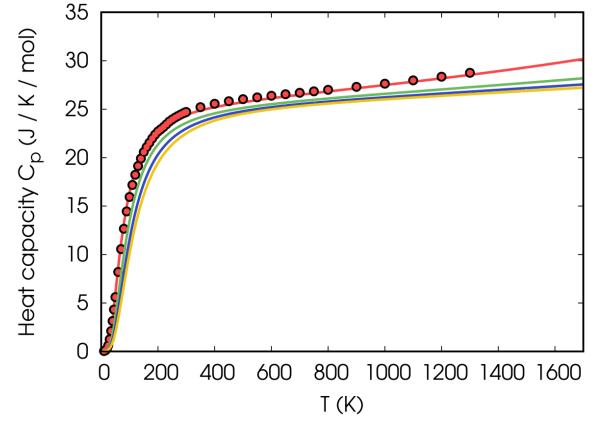

FIG. 4. Isobaric heat capacity per mole calculated in the present work at several pressures: 0 kbar (red), 500 kbar (green), 1000 kbar (blue), and 1500 kbar (yellow) compared with the experimental data at 0 kbar summarized in Ref. [1].

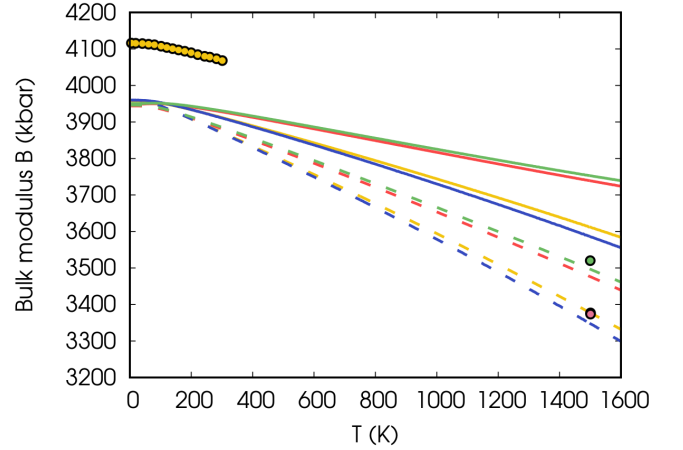

FIG. 5. PBE temperature variation of the bulk modulus at 0 kbar as obtained from the TDECs calculated within V-ZSISA QSA (red lines) and QHA (blue lines). The dashed lines are the isothermal values, while continuous lines represent the adiabatic values. The orange lines show the bulk modulus obtained from the EOS interpolation of the free energy along the stress-pressure curve. The green lines are the QSA bulk modulus obtained from QSA elastic constants (ECs) interpolated on all grid. The experimental data from Ref. [3] are shown as yellow dots. Blue (green) dots at 1500 K: isothermal QHA (QSA) results at the 1500 K geometry. Pink dots at 1500 K: isothermal QHA obtained with Fermi-Dirac occupations.

range.

Figs. 5 and 6 present a comparison between the calculated bulk modulus and experimental data. The distinction between these figures lies in the subtraction of the 0 K bulk modulus value in Fig. 6, thereby emphasizing the temperature dependence. The bulk modulus derived from ECs is compared with that obtained from the equation of state (EOS). Ideally, the EOS-derived

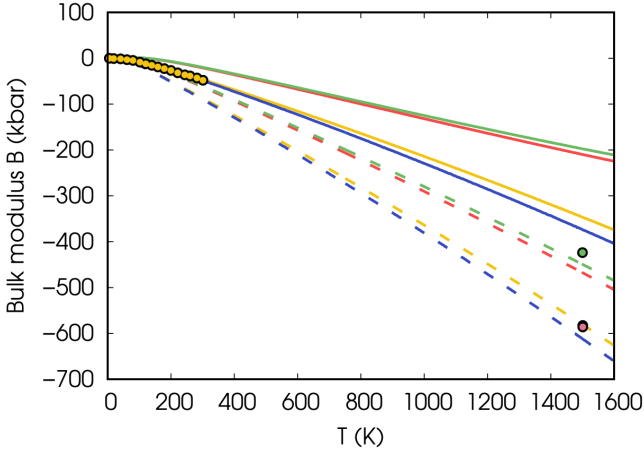

FIG. 6. Same data as shown in Fig. 5, with the 0 K values subtracted.

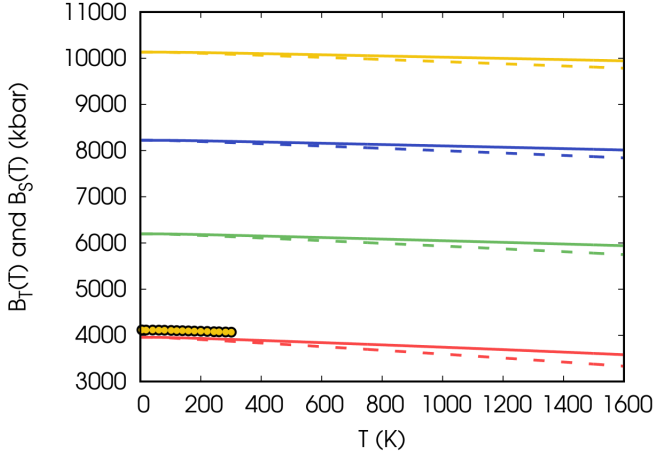

FIG. 7. PBE-calculated bulk modulus of osmium as a function of temperature at 0 kbar (red), 500 kbar (green), 1000 kbar (blue), and 1500 kbar (yellow). Results were obtained by interpolating the equation of state (EOS) derived from the free energy along the stress-pressure curve. Isothermal (dashed lines) and adiabatic (solid lines) bulk moduli are shown. Experimental adiabatic data at 0 kbar from Ref. [3] are plotted as yellow dots.

bulk modulus should align with the QHA bulk modulus. The observed discrepancy is attributed to the V-ZSISA. As demonstrated in the QSA calculations, where ECs can be computed both with and without V-ZSISA, the difference between the two approximations is similar to the difference between the bulk modulus derived from EOS and from V-ZSISA QHA ECs. Notably, the bulk modulus obtained from ECs calculated directly from free energy derivatives at 1500 K, without interpolation, precisely matches the isothermal bulk modulus derived from the EOS.

Fig. 7 presents the temperature dependent (adiabatic and isothermal) bulk moduli at several pressures (0 kbar, 500 kbar, 1000 kbar, and 1500 kbar).

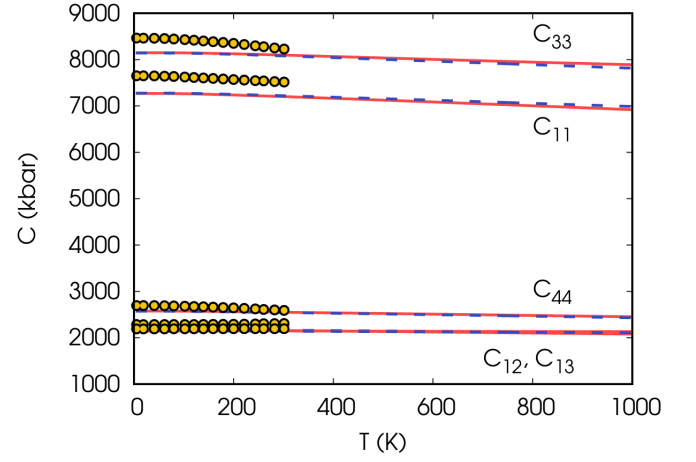

FIG. 8. QSA TDECs of osmium calculated within V-ZSISA (red continuous lines) and using the ECs on the full grid of values of  $a$  and  $c/a$  (blue dashed lines). The experimental data from Ref. [3] are shown as yellow dots.

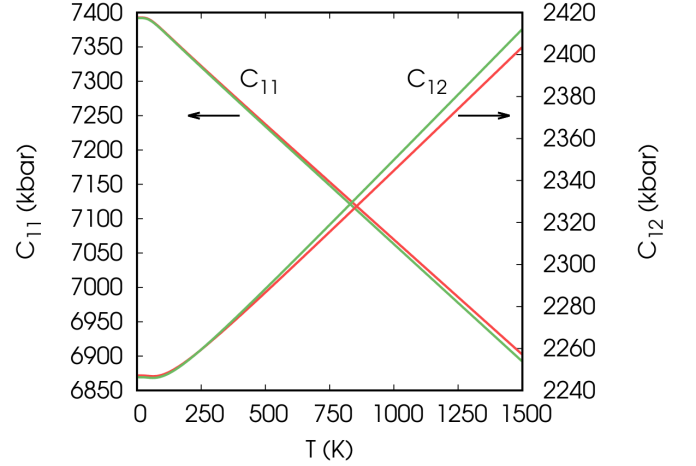

FIG. 9. QHA TDECs of osmium calculated within ZSISA (red lines) and using the full free-energy minimization (green line). The geometry is fixed to geometry number 6 in Table I.

Fig. 8 compares the QSA ECs calculated using the V-ZSISA approximation with those obtained from full grid interpolations. At the scale presented, the difference between the V-ZSISA and full grid results is minimal. As demonstrated in subsequent figures, discernible discrepancies become apparent only upon significant magnification.

Fig. 9 depicts the temperature variation of QHA  $C_{11}$  and  $C_{12}$  ECs which are the only ones influenced by atomic relaxations. These constants are calculated using ZSISA, with energy minimization, and also through full free energy minimization with respect to atomic coordinates. In this case, minor deviations are observable exclusively at the highest temperature investigated, 1500 K.

Figs. 10 through 14 display the ECs presented in the main paper, without subtracting the 0 K values. While

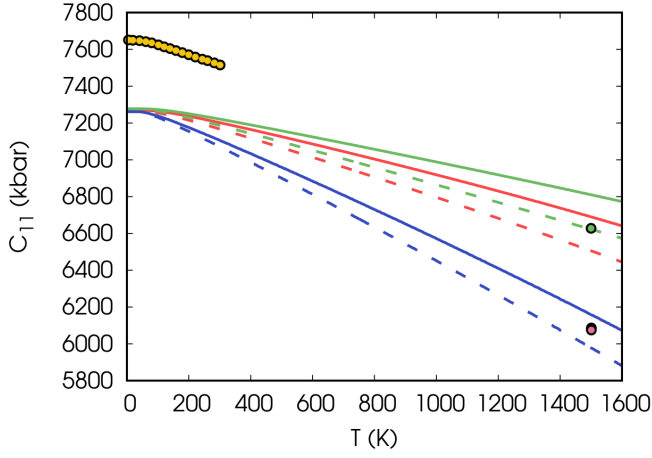

FIG. 10. PBE calculated temperature variation of osmium's  $C_{11}$  EC. Dashed lines represent isothermal ECs, while continuous lines show adiabatic ECs. Red curves correspond to the QSA within V-ZSISA, green curves to QSA interpolating over the entire grid, and blue curves to the V-ZSISA QHA calculation. Experimental data from Ref. [3] are shown with yellow circles. Blue (green) dots at 1500 K indicate isothermal QHA (QSA) results obtained at the 1500 K geometry. Pink dots at 1500 K represent isothermal QHA values calculated with Fermi-Dirac occupations.

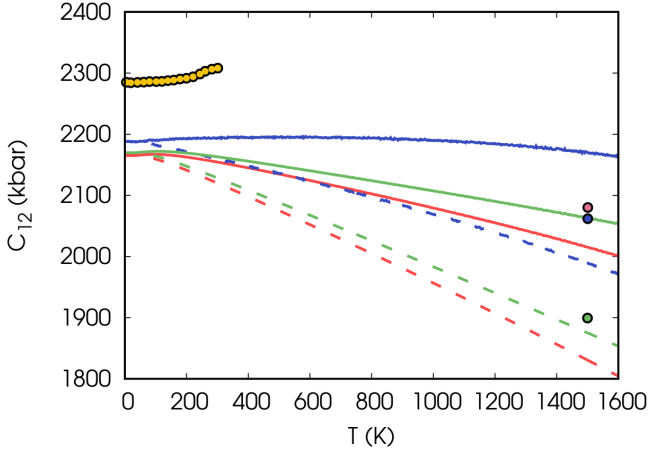

FIG. 11. PBE temperature variation of the  $C_{12}$  EC of osmium. The lines and dots have the same conventions of Fig. 10.

discerning the approximation that yields results closest to experimental data is more challenging in this representation, these figures are included for completeness.

Figs. 15 through 19 display the QHA V-ZSISA ECs as presented in the main paper, compared with the TDECs that we obtained when neglecting the electronic excitation contribution in the free-energy. These pictures show that this contribution, while quite small, gives a visible difference on the scale of these figures. Additionally, for comparative purposes, results from QHA calculations at the 1500 K geometry, incorporating the electronic exci-

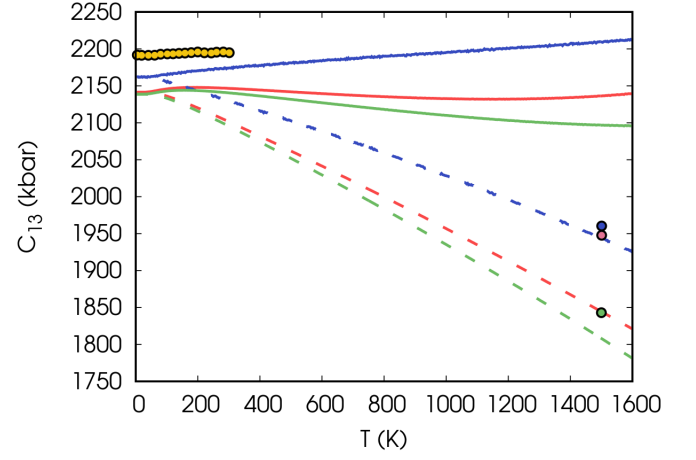

FIG. 12. PBE temperature variation of the  $C_{13}$  EC of osmium. The lines and dots have the same conventions of Fig. 10.

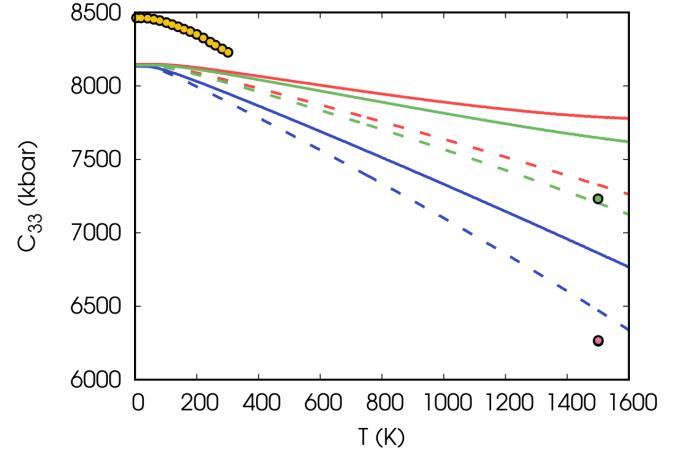

FIG. 13. PBE temperature variation of the  $C_{33}$  EC of osmium. The lines and dots have the same conventions of Fig. 10.

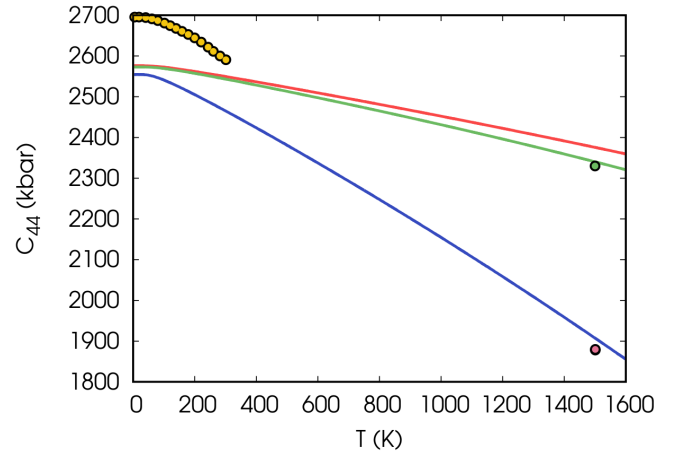

FIG. 14. PBE temperature variation of the  $C_{44}$  EC of osmium. The lines and dots have the same conventions of Fig. 10.

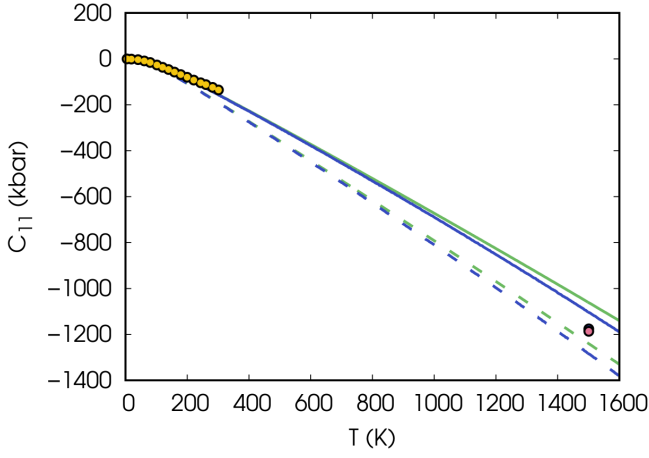

FIG. 15. PBE calculated temperature dependence of osmium's  $C_{11}$  EC. All curves are obtained within the V-ZSISA QHA calculation. Dashed lines represent isothermal ECs, while continuous lines denote adiabatic ECs. Blue curves include the contribution of electronic excitations in the free energy, whereas green curves neglect it. Experimental data from Ref. [3] are shown as yellow circles. The blue dot at 1500 K represents the isothermal QHA value at the 1500 K geometry, including electronic excitations. The pink dot illustrates where electronic excitation contributions have been incorporated into both the DFT calculation and phonon frequencies using Fermi-Dirac occupations at an electronic temperature of 1500 K.

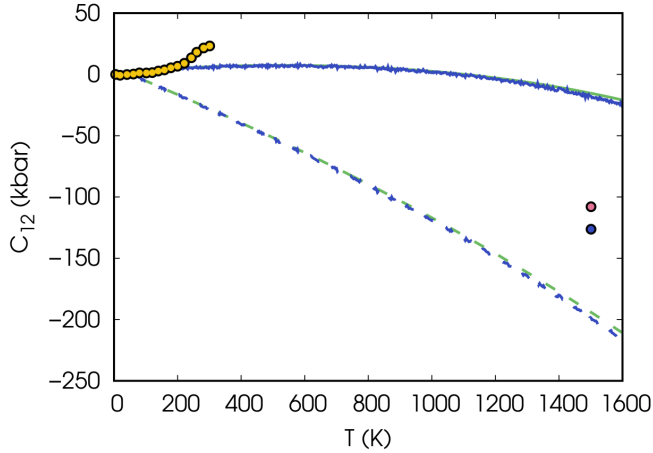

FIG. 16. PBE temperature variation of the  $C_{12}$  EC of osmium. The lines and dots have the same conventions of Fig. 15.

tation contribution to the free energy or utilizing Fermi-Dirac occupations (as presented in the main paper), are also included.

Fig. 20 shows the convergence of the elastic constants with the  $\mathbf{k}$  point grid used for the Brillouin zone interpolation.

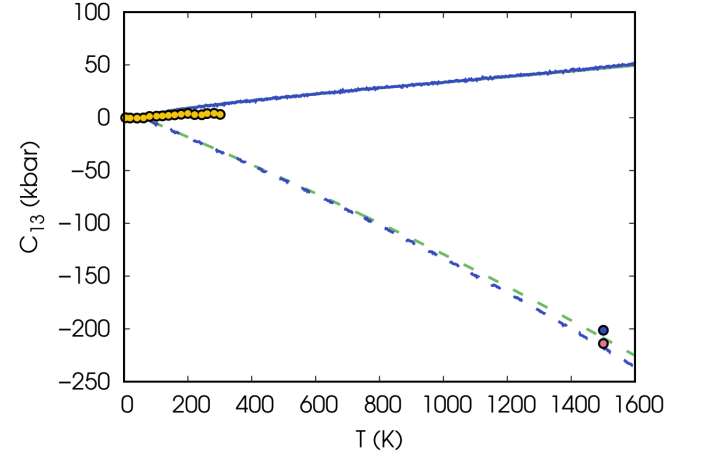

FIG. 17. PBE temperature variation of the  $C_{13}$  EC of osmium. The lines and dots have the same conventions of Fig. 15.

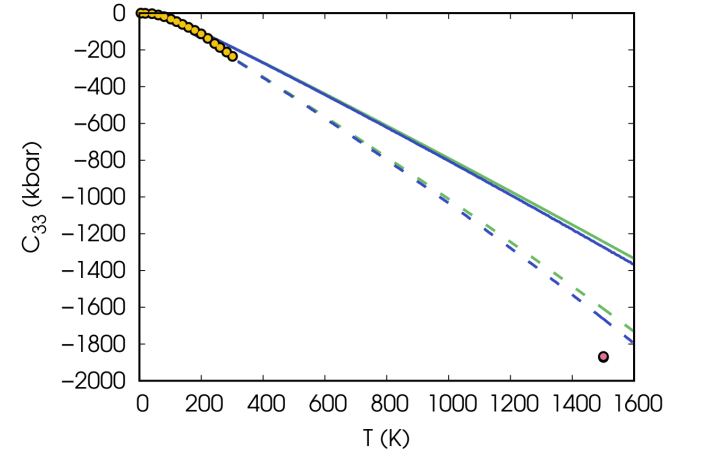

FIG. 18. PBE temperature variation of the  $C_{33}$  EC of osmium. The lines and dots have the same conventions of Fig. 15.

- 
- [1] J. W. Arblaster, Crystallographic Properties of Osmium: Assessment of properties from absolute zero to 1300 K, *Platinum Metals Review* **57**, 177 (2013).
  - [2] M. Palumbo and A. Dal Corso, Lattice dynamics and thermophysical properties of h.c.p. Os and Ru from the quasi-harmonic approximation, *Journal of Physics: Condensed Matter* **29**, 395401 (2017).
  - [3] C. Pantea, I. Stroe, H. Ledbetter, J. B. Betts, Y. Zhao, L. L. Daemen, H. Cynn, and A. Migliori, Elastic constants of osmium between 5 and 300 K, *Physical Review B* **80**, 024112 (2009).
  - [4] A. Dal Corso, Elastic constants of beryllium: a first-principles investigation, *Journal of Physics: Condensed Matter* **28**, 075401 (2016).

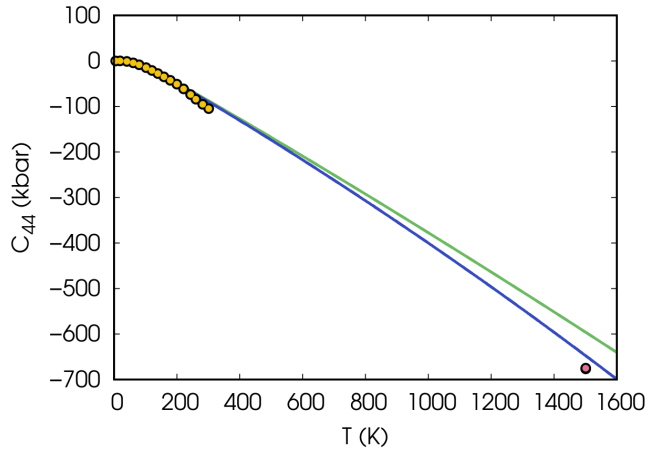

FIG. 19. PBE temperature variation of the  $C_{44}$  EC of osmium. The lines and dots have the same conventions of Fig. 15.

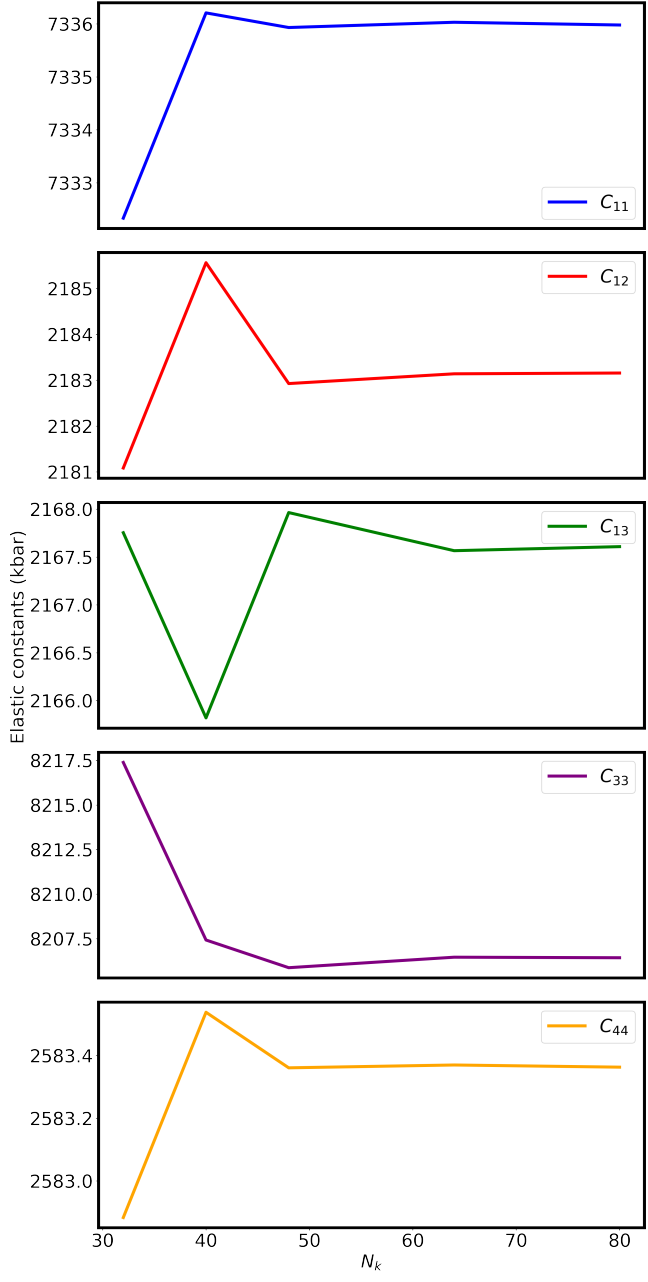

FIG. 20. Convergence of the  $C_{11}$ ,  $C_{12}$ ,  $C_{13}$ ,  $C_{33}$ ,  $C_{44}$  elastic constants with respect to the grid of  $\mathbf{k}$ -points used in the Brillouin zone integration. We used unshifted meshes  $(N_k, N_k, N_{k_z})$  described in Ref. [4] and plot the results as a function of  $N_k$ .
